# Supplementary material for: LogicVal:A Logic-Formalized Benchmark for Constraint Satisfaction in Text-to-Image Generation
Source: arXiv:2610.24051 source file (2026-10-16)
Supplement: Supplementary file 1 [file constraint_definitions.tex]

\newcommand{\fcore}[1]{%
  \begin{minipage}[t]{\linewidth}\centering\vspace{0pt}%
  $\begin{aligned}[t]#1\end{aligned}$%
  \end{minipage}}
\newcommand{\fcorewhere}[2]{%
  \begin{minipage}[t]{\linewidth}\centering\vspace{0pt}%
  $\begin{aligned}[t]#1\end{aligned}$\par\vspace{4pt}%
  {\tiny\textit{where:}\ $\begin{aligned}[t]#2\end{aligned}$}\par\vspace{2pt}%
  \end{minipage}}

\begin{table*}[p]
\centering
\scriptsize
\renewcommand{\arraystretch}{1.1}
\begin{tabularx}{\textwidth}{l >{\raggedright\arraybackslash}p{0.10\textwidth} >{\centering\arraybackslash}p{0.52\textwidth} >{\raggedright\arraybackslash}X}
\toprule
\textbf{ID} & \textbf{Name} & \textbf{Formal Core} & \textbf{Example} \\
\midrule
\multicolumn{4}{>{\columncolor{basecolor}}l}{\textbf{Object-Level Constraints}}\\
\addlinespace[2pt]
C1 & Existential Object
  & \fcore{\exists x\;\Phi_{prop}(x)}
  & [\textbf{positive literals only:}] There exists a blue sphere.\newline
    [\textbf{with negated literal:}] There exists a blue object that is not a sphere. \\
\addlinespace[2pt]
C2 & Universal Object
  & \fcore{\forall x\;\Phi_{prop}(x)}
  & [\textbf{positive literals only:}] All objects are blue spheres.\newline
    [\textbf{with negated literal:}] All objects are blue and not spheres. \\
\addlinespace[2pt]
C3 & Conditional Object
  & \fcore{\forall x\;\bigl(\Phi_{prop_1}(x)\rightarrow\Phi_{prop_2}(x)\bigr)}
  & [\textbf{positive literals only:}] All blue spheres are metal.\newline
    [\textbf{with negated literal:}] All blue spheres are not metal. \\
\midrule
\multicolumn{4}{>{\columncolor{basecolor}}l}{\textbf{SubGraph-Level Constraints}}\\
\addlinespace[2pt]
C4 & Existential
  & \fcorewhere{
      \exists x_1,\ldots,x_t\;\Bigl(\bigwedge\nolimits_{o=1}^{t}\Phi_{prop_o}(x_o)\wedge\mathrm{Rel}_{E}(x_1,\ldots,x_t)\Bigr)
    }{
      E &\subseteq\{(o,j)\mid 1\le o<j\le t\}
    }
  & [\textbf{positive literals only:}] There exists a blue sphere behind a red cube that is in front of a yellow cylinder.\newline
    [\textbf{with negated literal:}] There exists a blue sphere behind a red cube that is in front of a cylinder that is not yellow. \\
\addlinespace[2pt]
C5 & Conditional
  & \fcorewhere{
      &\forall x_1,\ldots,x_t\;\Bigl(\bigwedge\nolimits_{o=1}^{t}\Phi_{\mathrm{propCond}_o}(x_o)\wedge\mathrm{Rel}_{E_{\mathrm{cond}}}(x_1,\ldots,x_t)\\
      &\qquad\rightarrow\bigwedge\nolimits_{o=1}^{t}\Phi_{\mathrm{propReq}_o}(x_o)\wedge\mathrm{Rel}_{E_{\mathrm{req}}}(x_1,\ldots,x_t)\Bigr)
    }{
      E_{\mathrm{cond}},E_{\mathrm{req}} &\subseteq\{(o,j)\mid 1\le o<j\le t\}
    }
  & [\textbf{positive literals only:}] All blue spheres that are in front of red cubes are metal and behind yellow cylinders.\newline
    [\textbf{with negated literal:}] All blue spheres that are in front of cubes that are not red are not metal and behind cylinders that are not yellow. \\
\addlinespace[2pt]
C6 & Existential-Universal
  & \fcorewhere{
      &\exists x_1,\ldots,x_t\;\Bigl(\bigwedge\nolimits_{o=1}^{t}\Phi_{\mathrm{propSel}_o}(x_o)\wedge\mathrm{Rel}_{E_{\mathrm{sel}}}(x_1,\ldots,x_t)\\
      &\qquad\wedge\forall y_1,\ldots,y_m\;\Bigl(\bigwedge\nolimits_{v=1}^{m}\Phi_{\mathrm{propTar}_v}(y_v)\wedge\mathrm{Rel}_{E_{\mathrm{tar}}}(y_1,\ldots,y_m)\\
      &\qquad\qquad\rightarrow\mathrm{Rel}_{E_{\mathrm{req}}}(x_1,\ldots,x_t,y_1,\ldots,y_m)\Bigr)\Bigr)
    }{
      E_{\mathrm{sel}} &\subseteq\{(o,j)\mid 1\le o<j\le t\},\\
      E_{\mathrm{tar}} &\subseteq\{(v,w)\mid 1\le v<w\le m\},\\
      E_{\mathrm{req}} &\subseteq\{(o,v)\mid 1\le o\le t,\ 1\le v\le m\}
    }
  & [\textbf{positive literals only:}] There exists a blue sphere that is behind every red cube.\newline
    [\textbf{with negated literal:}] There exists a blue sphere that is behind every cube that is not red. \\
\addlinespace[2pt]
C7 & Universal-Existential
  & \fcorewhere{
      &\forall x_1,\ldots,x_t\;\Bigl(\bigwedge\nolimits_{o=1}^{t}\Phi_{\mathrm{propCond}_o}(x_o)\wedge\mathrm{Rel}_{E_{\mathrm{cond}}}(x_1,\ldots,x_t)\\
      &\qquad\rightarrow\exists y_1,\ldots,y_m\;\Bigl(\bigwedge\nolimits_{v=1}^{m}\Phi_{\mathrm{propWit}_v}(y_v)\wedge\mathrm{Rel}_{E_{\mathrm{wit}}}(y_1,\ldots,y_m)\\
      &\qquad\qquad\wedge\mathrm{Rel}_{E_{\mathrm{req}}}(x_1,\ldots,x_t,y_1,\ldots,y_m)\Bigr)\Bigr)
    }{
      E_{\mathrm{cond}} &\subseteq\{(o,j)\mid 1\le o<j\le t\},\\
      E_{\mathrm{wit}} &\subseteq\{(v,w)\mid 1\le v<w\le m\},\\
      E_{\mathrm{req}} &\subseteq\{(o,v)\mid 1\le o\le t,\ 1\le v\le m\}
    }
  & [\textbf{positive literals only:}] Every blue sphere that is in front of a yellow cylinder has some red cube behind it.\newline
    [\textbf{with negated literal:}] Every blue sphere that is in front of a cylinder that is not yellow has some cube that is not red behind it. \\
\midrule
\multicolumn{4}{>{\columncolor{basecolor}}l}{\textbf{Cardinality-Level Constraints}}\\
\addlinespace[2pt]
C8 & Cardinality
  & \fcorewhere{
      \biggl|\biggl\{x_1\;\Big|\;\exists x_2,\ldots,x_t\;\Bigl(\bigwedge\nolimits_{o=1}^{t}\Phi_{\mathrm{prop}_o}(x_o)\wedge\mathrm{Rel}_{E}(x_1,\ldots,x_t)\Bigr)\biggr\}\biggr|\;\theta\;k
    }{
      E &\subseteq\{(o,j)\mid 1\le o<j\le t\},\\
      \theta &\in\{=,\neq,<,\le,>,\ge\},\quad k\in\mathbb{N}
    }
  & [\textbf{object count:}] There are exactly three blue spheres.\newline
    [\textbf{contextual object count:}] There are exactly three blue spheres that are in front of some red cube. \\
\addlinespace[2pt]
C9 & Aggregate Comparison
  & \fcorewhere{
      \begin{gathered}
      \biggl|\biggl\{x_1\;\Big|\;\exists x_2,\ldots,x_t\;\Bigl(\bigwedge\nolimits_{o=1}^{t}\Phi_{\mathrm{prop}_o}(x_o)\wedge\mathrm{Rel}_{E_x}(x_1,\ldots,x_t)\Bigr)\biggr\}\biggr|\\
      \theta\\
      \biggl|\biggl\{y_1\;\Big|\;\exists y_2,\ldots,y_m\;\Bigl(\bigwedge\nolimits_{v=1}^{m}\Phi_{\mathrm{prop}'_v}(y_v)\wedge\mathrm{Rel}_{E_y}(y_1,\ldots,y_m)\Bigr)\biggr\}\biggr|
      \end{gathered}
    }{
      E_x &\subseteq\{(o,j)\mid 1\le o<j\le t\},\\
      E_y &\subseteq\{(v,w)\mid 1\le v<w\le m\},\\
      \theta &\in\{=,\neq,<,\le,>,\ge\}
    }
  & [\textbf{object-count comparison:}] The number of blue spheres equals the number of red cubes.\newline
    [\textbf{contextual comparison:}] The number of blue spheres that are in front of some red cube is greater than the number of yellow cylinders. \\
\bottomrule
\end{tabularx}
\caption{Primitive logical constraint classes ordered by increasing logical expressivity. The notation used in the formal cores is defined in the formalization conventions above; below each formula are the admissible index pairs of its relational patterns.}
\label{tab:constraint-classes}
\end{table*}



\section{Formal Definitions of the Constraint Classes}
\label{app:taxonomy}

\paragraph{Formalization conventions.}
We use the following notation in Table~\ref{tab:constraint-classes}.

\begin{itemize}
    \item \textbf{Objects.}
    The variables $x_1,\ldots,x_t$ and $y_1,\ldots,y_m$ range over the objects of a scene.

    \item \textbf{Object descriptions.}
    An attribute literal is a unary predicate for an attribute value, positive or negated, e.g.\ $\mathit{Blue}(x)$ or $\neg\mathit{Sphere}(x)$.
    An object description $\Phi_{prop}(x)$ is a conjunction of attribute literals, e.g.\ $\mathit{Blue}(x)\wedge\neg\mathit{Sphere}(x)$; an empty description is always true.
    The subscript only names the description (e.g.\ $\Phi_{prop_1}$, $\Phi_{\mathrm{propCond}_o}$), so different subscripts denote different descriptions.

    \item \textbf{Relational patterns.}
    A relational literal is a spatial relation between two objects, positive or negated, e.g.\ $\mathit{Behind}(x_1,x_2)$ or $\neg\mathit{Left}(x_1,x_2)$.
    For variables $z_1,\ldots,z_r$ and a set of index pairs $E$, the pattern
    \[
        \mathrm{Rel}_{E}(z_1,\ldots,z_r)=\bigwedge_{(i,j)\in E} M_{ij}(z_i,z_j)
    \]
    is a conjunction of relational literals $M_{ij}$, one for each related pair; if $E=\emptyset$, it is always true.
    In C6 and C7, $\mathrm{Rel}_{E_{\mathrm{req}}}$ relates the two groups, i.e.\ each $(o,v)\in E_{\mathrm{req}}$ gives a literal $M_{ov}(x_o,y_v)$.
    The subscript of $E$ only names the role of the pattern: condition ($\mathrm{cond}$), requirement ($\mathrm{req}$), selected object ($\mathrm{sel}$), universal target ($\mathrm{tar}$) or existential witness ($\mathrm{wit}$).

    \item \textbf{Counting.}
    In C8 and C9, $\bigl|\{x_1\mid\exists x_2,\ldots,x_t\;\psi\}\bigr|$ is the number of objects $x_1$ for which some $x_2,\ldots,x_t$ satisfy $\psi$; the other variables only give context and are not counted.
    The count is compared with $\theta\in\{=,\neq,<,\leq,>,\geq\}$.
\end{itemize}



Each class is implemented by several ASP templates; Appendix~\ref{app:templates} lists them with their encodings.
